# Supplementary material for: Mapping of Yu-Shiba-Rusinov states from an extended scatterer
Source: arXiv:1807.00646 source file (2018-07-02)
Supplement: Supplementary file 1 [file SI_CuPc-28-06-05.pdf]

# Supplementary Information:

# Mapping of Yu-Shiba-Rusinov states from an extended scatterer


Markus Etzkorn,[1,*,†] Matthias Eltschka,[1,†] Berthold Jäck,[1] Christian R. Ast,[1] and Klaus Kern[1,2]

[1]*Max-Planck-Institut für Festkörperforschung, 70569 Stuttgart, Germany*

[2]*Physique de la Matière Condensée, Ecole Polytechnique Fédérale de Lausanne, 1015 Lausanne, Switzerland*



(Dated: June 28, 2018)

## INFLUENCE OF THE ADSORPTION SITE ON THE YSR STATES

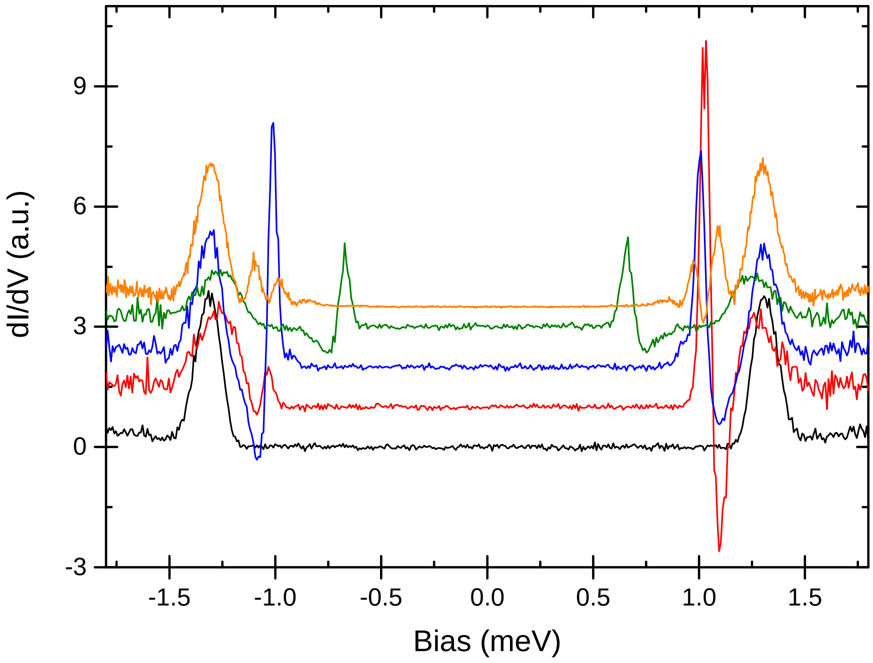


FIG. 1. Collection of different spectra measured on different CuPc molecules, the black line is a spectrum measured on the pure vanadium surface for comparison. The spectra are selected specifically to show the large variety of different YSR signatures. Different number of YSR states with different energies, spectral intensities and particle-hole asymmetries are observed. The spectra are shifted in the y-direction for clarity.

In Figure S1 different spectra obtained on different molecules and in a clean Vanadium-Vanadium-Junction (black) are shown to display the sensitivity of YSR states on the molecule adsorption site on the V$(5 \times 1)$ reconstruction. They are selected to illustrate the rich variety of spectra changing the number of (resolved) YSR states, their energy position, spectral intensity and particle-hole asymmetry observed on different molecules. We attribute the changes of the YSR states to the different adsorption conformations and accompanied different interactions with the superconducting substrate. However, YSR spectra similar to the ones discussed in the main text or shown in the blue and red spectra in Fig. S1 are most frequently found.

## FITTING PROCEDURE

We have first fitted the spectra of the pure V-V junction following the routine described in Ref [1, 2]. We include the influence of the electron-photon interaction during the tunneling process through the $P(E)$-function [3]. The necessary parameters to include the influence of the electromagnetic environment are obtained from measurements of the Josephson effect [1, 2] on the very same junction. In short, the Josephson current flowing through in a junction with small capacitance can at each voltage V be calculated as $I(V) = \frac{\pi\hbar}{4e} I_0[P(2e \cdot V) - P(-2e \cdot V)]$, where $I_0$ is the Josephson critical current and $P(2e \cdot V)$ is the probability function of a photon exchange (with energy $E = 2e \cdot V$) with the electromagnetic environment [4]. The $P(E)$ function can be modeled using its capacity $(C_J)$, its effective temperature $(\mathrm{T_{eff}})$, the resonance energy $(\omega_{\mathrm{res}})$ and quality factor (q) of the electromagnetic environment. A fit of the Josephson current measured with the same tip as used in the experiments is shown in Fig. S2. As pointed out in Refs [1, 2] in detail, we are able to accurately determine the parameters describing the electromagnetic environment from such Josephson measurements, which in return allows us to precisely determine the energy resolution of the experiment.

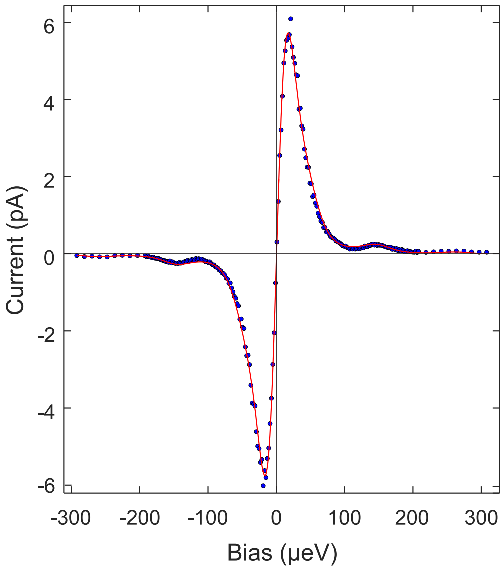


FIG. 2. Josephson current measured with the same V tip on the V substrate at $T = 15$ mK. The red line is a fit to the data with using the P(E) function as described in the text, with $\mathrm{C_J} = 9.25\,\mathrm{fF}$, $\mathrm{T_{eff}} = 0.1\,\mathrm{K}$, $\omega_{\mathrm{res}} = 124\,\mu\mathrm{eV}$, and $\mathrm{q} = 0.48$.

The superconducting density of states of tip and sample have been modeled with the Maki

theory which in the absence of magnetic field is given by [5–8]:

$$\rho(E) = \frac{\rho_0}{2} \operatorname{sgn}(E) \operatorname{Re}\left(\frac{u}{\sqrt{u^2-1}}\right) \tag{1}$$

with $\rho_0$ being the normal conducting density of states and u given by:

$$u = \frac{E}{\Delta} + \zeta \frac{u}{\sqrt{1-u^2}} \tag{2}$$

where $\zeta$ is a measure of the orbital depairing (the values used for the fits are ($\zeta_{tip} = 0.0172$) and ($\zeta_{sample} = 0.005$)). In addition, a Dynes like parameter ($E \to E - i\Gamma$) was included to account for the observed broad quasiparticle coherence peaks [7, 8]. We always find the order parameter of the tip to be reduced compared to the Vanadium bulk gap value $\Delta_{sample} = 760\,\mu\text{eV}$ [8]. For the tips used in these experiments the gap value was found to be $\Delta_{tip} = 570\,\mu\text{eV}$ and $590\,\mu\text{eV}$, respectively; likely due to confinement effects at the tip apex [8]. The YSR states have been modeled using Lorentz curves with small (constant) full width half maximum of $w = 10\,\mu\text{eV}$. This intrinsic width so small that the spectral shape of the YSR peaks is purely determined by the energy resolution of the experiment resulting from the energy exchange of the tunneling electrons with the electromagnetic environment as described above. For all fits shown in the paper, we consider a single electron tunneling process to populate the YSR-state, which explicitly assumes a decay channel sufficiently effective to on average reach equilibrium population before the next electron tunnels through the junction [9]. A detailed discussion on the justification of this assumption is made in the following paragraph.

## SINGLE VERSUS MULTIPLE TUNNELING CONTRIBUTIONS TO THE YSR PEAK INTENSITIES AND ESTIMATION OF THE INTRINSIC LIFE TIME BROADENING

In the main text, we have explicitly assumed that the dominant transport channel in the measurements of YSR states is via single electron tunneling. It has been shown that at high enough conductances multiple tunneling processes can play an important role in the transport [9]. For example an electron may tunnel into a particle YSR state and a hole tunnels back from the hole like YSR state, depopulating the YSR state by injecting a Cooper pair in the sample. This essentially will lead to a different spectral appearance of the YSR states and a non-linear dependence of the spectral peak height on the underlying YSR wave function. The hallmark of dominant single

particle tunneling in spectra measured with a superconducting tip in a negative differential conductance on the high energy side of the YSR peak, that results from the convolution of a Lorentzian peak with a BCS like density of states. In multiple tunneling processes this feature is absent [9]. As already mentioned, we find clear negative differential conductance features on the high energy side of the YSR states expected for single particle tunneling processes (compare to Ref. [9]) and therefore, negligible multiple tunneling contributions. Though the experimental evidence is clear, it requires an effective, temperature independent decay channel for the electron populating the YSR state. Dominating single particle tunneling requires the time to deexcite a YSR state to be much shorter than the average time between two tunneling events. Since the overlap in the wave functions between impurity and sample will be many orders of magnitude larger than between the impurity and the tip states (under typical tunneling conditions), it is easy to see that a sample density of states many orders of magnitude smaller than the YSR intensity will be sufficient to provide enough decay channels. Therefore, small deviations from a BCS like density of states that lead to a finite number of quasiparticle excitations in the gap of the superconducting V sample will provide an efficient pathway to deexcite YSR state into the continuum of quasiparticle excitations with a low or even no energy barriers to overcome.

The width of the YSR peaks in our measurements are dominated by the experimental energy resolution. Following Ref. [9], we can, nevertheless, estimate the energy scale expected for multiple tunneling processes to be $\approx 3\,\mu\mathrm{eV}$ in our measurements and therefore the intrinsic life time broadening must be much larger than this value. Our data is, therefore, in full agreement with an intrinsic lifetime broadening of the YSR states of $10 \pm 5\,\mu\mathrm{eV}$ resulting from single electron tunneling with a decay channel into remaining single particle states within the gap of the V substrate.

## POINT SCATTERING MODEL

For the case of an isotropic band structure with a Fermi wave vector $k_F$ and a point scattering impurity with a classical spin the YSR wave functions are given by [10–13]::

$$\Psi^{(\pm)}(r) \propto \frac{\sin\left(k_F r - \delta^{\pm}\right)}{k_F r} \exp\left(-r\left|\sin\left(\delta^{+} - \delta^{-}\right)\right| / \xi_0\right) , \tag{3}$$

where $\pm$ indicate YSR states with particle and hole character, $\delta^{\pm}$ is the phase shift resulting from the scattering and and $\xi_0$ is the coherence length of the superconductor. In particular, the observed phase difference between the particle and hole wavefunctions correspond to the observed

energies ($E_i$) of the YSR states with which they are related by [10, 14]:

$$\frac{E_i}{\Delta} = \cos\left(\delta_i^+ - \delta_i^-\right). \quad (4)$$

This phase difference is caused by a breaking of the particle-hole symmetry which can result from a Coulomb contribution to the scattering potential according to [10, 15]:

$$\tan\left(\delta^{\pm}\right) = (\pi N_0)\,(V \pm JS/2)\,, \quad (5)$$

where $N_0$ is the density of states at $E_F$ in the normal state and $V$ and $JS/2$ are the Coulomb and exchange scattering potential, respectively. In the two experimental studies discussing the spatial evolution of the YSR states, the scattering impurity was a single $3d$-transition metal impurity [13, 14], for which the central assumption of a point scattering potential ($i.e.$ the spatial extent of the potential to be much smaller than $\lambda_F$) is reasonable.

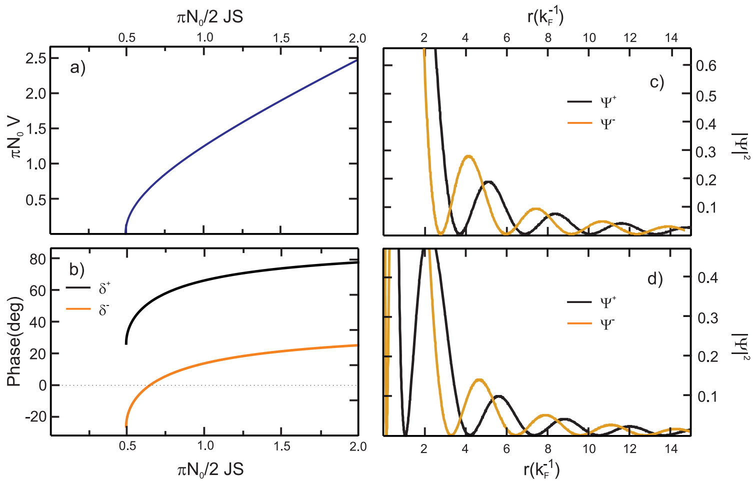


FIG. 3. a) Combinations of exchange (JS) and potential (V) scattering strength that fulfill equation (S5) for an energy of $E = 465\,\mu$eV. b) Solutions for the scattering phases as given by equation (S4) as function of the exchange scattering potential strength. Note that according to the equation the difference between the two scattering phase remains constant.c)-d) Spatial dependance of the probability density of the particle and hole wave functions for $E = 465\,\mu$eV and $\frac{\pi N_0}{2} JS = 0.5$ (c) and 1 (d), respectively.

Figure S3 a) shows the size of the potential and exchange scattering that is needed to create YSR states with the energy of $465\,\mu$eV and $490\,\mu$eV. Figure S3 b) then shows the according phases fulfilling equation S4 and S5. Figure S3 c) and d) show YSR state intensities with particle and hole character as they are expected to arise from equation S3 for two different values of exchange

scattering potential. A strong phase difference is expected that is not seen in the experiment. This illustrates that in contrast to the literature published YSR states created by atomic impurities, our data can not be explained by this simple model, which is a direct consequence of the extended scattering potential that is created by the molecule.

## 2D MAPS OF THE YSR INTENSITIES FOR THE SECOND MOLECULE

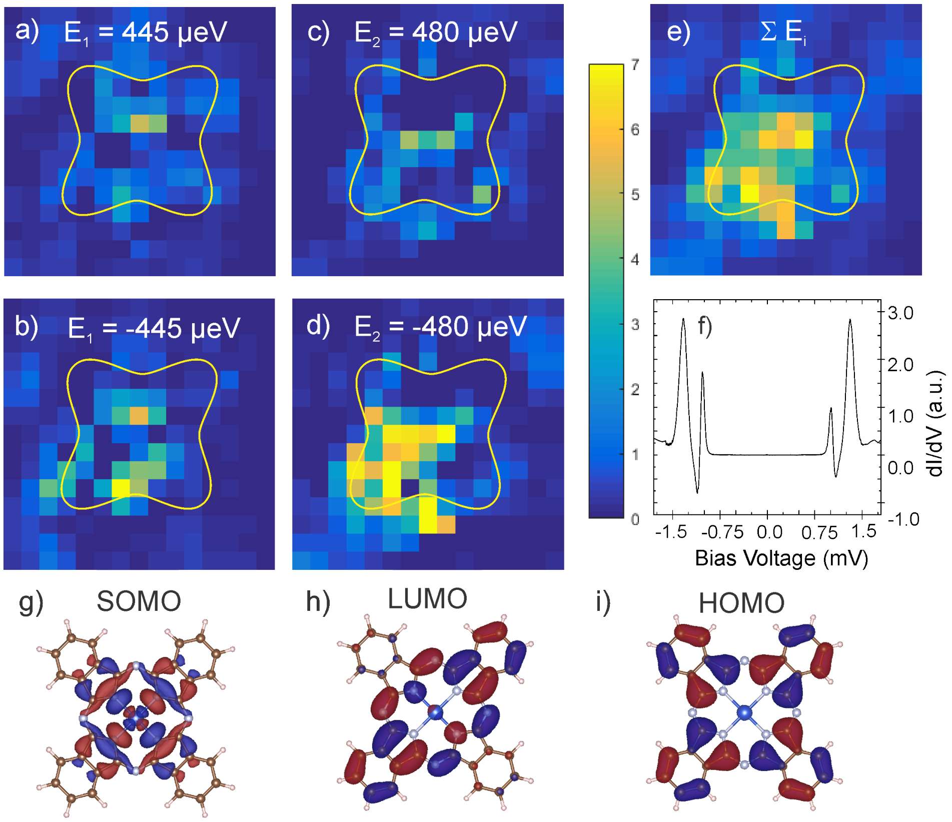


FIG. 4. a)-d) show the two dimensional distribution of the YSR intensities for particle (a) and hole (b) states at $E = 445\,\mu eV$ and particle (c) and hole (d) states at $480\,\mu eV$, respectively. The contour of the molecule is inserted. Note that the local minima in a) and b) and the maxima in c) and d) are found not in the Cu center but towards the pyrrolic N on one of ligands. This is also clearly seen in the two dimensional sum over all YSR peaks shown in e). f) Average spectrum obtained by summation over all spectra of the 2D map. A clear particle hole asymmetry is visible. g)-i) molecular orbitals as shown in the main text added for comparison.

We have measured a grid of 25 $\times$ 25 spectra over the molecule for which the line of spectra have been shown in figure 3 in the main text. Following the same analysis as discussed before we have extracted the 2D spatial variations of the YSR-state intensities, which is shown in Fig. S 4. We find a clear correspondence of these results to the intensities maps shown in the main text. The two dimensional distribution of the YSR states over the molecule reveals a clear shift of the spectral intensity to one of the four ligands which reflects the broken symmetry of the molecule due to the adsorption conformation, similar to the results discussed on the other molecule. Like in the measurements discussed in Fig. 2 of the main text, the lowest energy state is localized close to the center of molecule on one pyrrolic N-atom, while the higher energy state is more delocalized and have more spectral weight on the organic ligands of the molecule. It may well be that the higher energy YSR state measured on molecule is actually composed of two YSR states that are separated by too small an energy to be resolved (in which case the structure would be very close to the other molecule discussed in the main text). The spectral weight of the sum of all YSR states (Fig. S4 e)) is again shifted away from the metal center towards one ligand (note that in Fig. S4 the molecule is rotated by $45^\circ$ as compared to Fig. 2 in the main text), but again at least some spectral weight is also found on the other organic ligands. The sum over all spectra shown in Fig. S4 f) also reveals a clear particle hole asymmetry of the YSR state intensities.

---

* Corresponding author; electronic address: m.etzkorn@tu-bs.de; Present address: Insitut für Angewandte Physik, TU Braunschweig.

† These two authors contributed equally.

[1] B. Jäck *et al.*, *Phys. Rev. B* **93**, 020504(R) (2015).

[2] C. R. Ast *et al.*, *Nat. Com.* **7**, 13009 (2016).

[3] M. H. Devoret *et al.*, *Phys. Rev. Lett.* **64**, 1824 (1990).

[4] G.-L. Ingold, H. Grabert and U. Eberhardt, *Phys. Rev. B* **50**, 395 (1994).

[5] K. Maki, *Prog. Theor. Phys.* **32**, 29 (1964).

[6] D. C. Worledge and T. H. Geballe, *Phys. Rev. B* **62**, 447 (2000).

[7] R. C. Dynes, V. Narayanamurti and J. P. Garno, *Phys. Rev. Lett.* **41**, 1509 (1978).

[8] M. Eltschka *et al.*, *Applied Physics Letters* **107**, 122601 (2015).

[9] M. Ruby *et al.*, *Phys. Rev. Lett.* **115**, 087001 (2015).

[10] A. V. Balatsky, I. Vekhter and J.-X. Zhu, *Rev. Mod. Phys.* **78**, 373 (2006).

[11] A. Yazdani, B. A. Jones, C. P. Lutz, M. F. Crommie and D. M. Eigler, *Science* **275**, 1767 (1997).

[12] E. W. Hudson *et al.*, *Nature* **411**, 920 (2001).

[13] G. C. Ménard *et al.*, *Nat. Phys.* **11**, 1013 (2015).

[14] M. Ruby, Y. Peng, F. von Oppen, B. W. Heinrich and K. J. Franke, *Phys. Rev. Lett.* **117**, 186801 (2016).

[15] A. I. Rusinov, *J. Exp. Theor. Phys.* **9**, 85 (1969).
